# Supplementary material for: Telling stories with data -- A systematic review
Source: arXiv:2312.01164 source file (2023-12-02)
Supplement: Supplementary file 1 [file 45_appendix_effects.tex]

\subsection{List of effects from empirical studies}

% Please add the following required packages to your document preamble:

% Note: It may be necessary to compile the document several times to get a multi-page table to line up properly

\begin{landscape}
\begin{longtable}[c]{@{}p{3.5cm}p{4.5cm}clccp{2.4cm}ll@{}}
\caption{Overview of all dependent and independent variables in papers that contained empirical studies on the effects of storytelling}
\label{tab:hci_overview}\\
\toprule
Dep. variable & Ind. variable & Effect & Method & Lab & Wild & Sample sizes & Papers \\* \midrule
\endfirsthead
\toprule
Dep. variable & Ind. variable & Effect & Method & Lab & Wild & Sample sizes & Papers \\* \midrule
\endhead
Accuracy   & Data comic & 0  & mixed-method  &  \checkmark   &      &  medium--large    &\cite{43wang2019comparing} \\
Aesthetics  & Visual cue types & +/- & quantitative & \checkmark  &  & medium--large & \cite{307kong2019understanding} \\
Aesthetics  & data visualization & +/- & quantitative &   & \checkmark & small & \cite{317tang2020design} \\
Attitude & Added empathy conditions & + & quantitative &  & \checkmark & medium & \cite{326liem2020structure} \\
Attitude & Interaction technique & 0 & quantitative &  & \checkmark & medium & \cite{327heyer2020pushing} \\
Attitude & Data representation & + & quantitative & \checkmark & & medium & \cite{327heyer2020pushing} \\
Attention  & News visualizations & + & mixed-method  & \checkmark  &  & large &\cite{185de2018does} \\
Awareness & Static map visualization & + & quantitative & \checkmark & & small & \cite{359burkhard2005tube} \\
Awareness & Storytelling visualization & + & quantitative &  & \checkmark & large & \cite{so2020humane} \\
Cognitive load & Layout of infographics & + & eye-tracking / experimental & \checkmark & & small & \cite{289majooni2018eye} \\
Communicativeness & Interactive visualization  &+  & quantitative & \checkmark &  &medium  &\cite{70lunterova2019explorative} \\
Comprehension &  Interpretation and recall & + & quantitative &  \checkmark  & & medium &\cite{302obie2019study} \\
Comprehension  & Visual cue types & 0 & quantitative & \checkmark  &  & medium--large & \cite{307kong2019understanding} \\
Comprehension & Slideshow layout  & + & quantitative  & \checkmark   &   & large    &\cite{103zhi2019linking} \\
Comprehension & author driven narratives in visualizations  & + & qualitative and quantitative  & \checkmark   &   & medium    &\cite{obie2020effect} \\
Data wrangling strategies    & Learning environment    & +     & qualitative  & \checkmark  &       & small      &\cite{52jiang2019data} \\
Depth of exploration & Trivia game elements & + & quantitative &  & \checkmark & NA, online views & \cite{081diakopoulos2010game}\\
Ease of Use & Video and annotated visualization  & +  & mixed-method  & \checkmark  &  & small     &\cite{82zhi2019gameviews} \\
Efficiency in exploring data & VIStory, interactive storyboard & + & qualitative / quantitative & \checkmark & & medium & \cite{174zeng2020vistory}  \\
Effectiveness    & Feature-driven animation  & +  & quantitative   & \checkmark  &   & small  & \cite{63yu2016effectiveness} \\
Effectiveness   & Narration \& interactive slides  & +  & quantitative  & \checkmark  &       & small  & \cite{264wang2016guided} \\ 
Enjoyment & Video and annotated visualization  & +  & mixed-method  & \checkmark  &  & small     &\cite{82zhi2019gameviews} \\
Enjoyment    & Data comic & +  & mixed-method  &  \checkmark   &      &  medium--large    &\cite{43wang2019comparing} \\
Engagement  & Static map visualization & + & quantitative & \checkmark & & small & \cite{359burkhard2005tube} \\
Engagement & Video and annotated visualization  & +  & mixed-method  & \checkmark  &  & small     &\cite{82zhi2019gameviews} \\
Engagement    & Data comic & +  & mixed-method  &     &   \checkmark   &  medium--large    &\cite{43wang2019comparing} \\
Engagement & Linking  & + & quantitative  & \checkmark   &   & large    &\cite{103zhi2019linking} \\
Engagement & Storytelling in visualizations  & + & focus group  & \checkmark   &   & large    &\cite{234figueiras2014tell} \\
Engagement & content and design of storylines  & + & mixed method  & \checkmark   &   & medium   &\cite{135arevalo2020storylines} \\
Engagement & narrative visualization techniques  & 0 & quantitative  &    & \checkmark  & large  &\cite{143boy2015storytelling} \\
Engagement & personalised story  & 0 & mixed-method  &    & \checkmark  & medium  &\cite{356concannon2020brooke} \\
Engagement & Interactive story & + & qualitative  &     &  \checkmark    & large    &\cite{meuschke2022narrative} \\
Engagement & home and public setting &  & mixed method  &  \checkmark    &  \checkmark    & small    &\cite{van2022more} \\
Focus & Graphs with(out)background stories  & + & quantitative  & \checkmark   &   & large  &\cite{zhao2021evaluating} \\
Information retrieval & Story graph visualisation approach & + & experimental & \checkmark & & medium & \cite{019schumann2013approach} \\
Information retrieval & Graphs with(out)background stories & + & quantitative & \checkmark & & large & \cite{zhao2021evaluating} \\
Insights & Static map visualization & + & quantitative & \checkmark & & small & \cite{359burkhard2005tube} \\
Interaction & Linking  & + & quantitative  & \checkmark   &   & large    &\cite{103zhi2019linking} \\
Interpretation & Visual expressiveness, annotations & + & qualitative & \checkmark &  & medium & \cite{155bach2016telling} \\
Interpretation & Familiarity, story context & + & qualitative & \checkmark &  & medium & \cite{155bach2016telling} \\
Interpretation & Visualizations with story elements & + & qualitative & \checkmark &  & large & \cite{fernandez2021storytelling} \\
Interpretation & Visualizations with context information & + & experimental &  & \checkmark & large & \cite{mantri2022viewers} \\
Likeability & Various storytelling elements & + & qualitative / experimental & \checkmark & & small & \cite{235figuerias2014narrative} \\
Memorability  &  Interpretation and recall & - & quantitative &  \checkmark  & & medium &\cite{302obie2019study} \\
Memorability    & Data comic & - & mixed-method  &  \checkmark   &      &  medium--large    &\cite{43wang2019comparing} \\
Memorability & Interactive story & + & qualitative  &     &  \checkmark    & large    &\cite{meuschke2022narrative} \\
Message credibility & Statistical information and data visualization & + & experimental  &     &  \checkmark    & large    &\cite{link2021credibility} \\
Navigation & Various storytelling elements & + & qualitative / experimental & \checkmark & & small & \cite{235figuerias2014narrative} \\
Recall  & Static map visualization & + & quantitative & \checkmark & & small & \cite{359burkhard2005tube} \\
Recall  & Interactive visualization & 0 & quantitative & \checkmark & & medium & \cite{302obie2019study} \\
Recall  & Visual cue types & 0 & quantitative & \checkmark  &  & medium--large & \cite{307kong2019understanding} \\
Recall & Slideshow layout and linking  & + & quantitative  & \checkmark   &   & large    &\cite{103zhi2019linking} \\
Recall & author driven narratives in visualizations  & + & qualitative and quantitative  & \checkmark   &   & medium    &\cite{obie2020effect} \\
Recall & data storytelling visualizations  & + & experimental  & \checkmark   &   & large   &\cite{zdanovic2022influence} \\
Reading experience & Interactivity & + & experimental  &     &  \checkmark    & large    &\cite{link2021credibility} \\
Time spent reading& Linking  & + & quantitative  & \checkmark   &   & large    &\cite{103zhi2019linking} \\
Understanding & Annotated charts & + & qualitative & \checkmark & & small & \cite{235figuerias2014narrative} \\
Understanding & Static map visualization & + & quantitative & \checkmark & & small & \cite{359burkhard2005tube} \\
Understanding & Various storytelling elements & + & qualitative / experimental & \checkmark & & small & \cite{235figuerias2014narrative} \\
Understanding & Layout of infographics & + & eye-tracking / experimental & \checkmark & & small & \cite{289majooni2018eye} \\
Understanding & Interactive visualization & + & quantitative & \checkmark & & medium & \cite{302obie2019study} \\
Understanding & Interactive visualization & + & qualitative & \checkmark & & medium & \cite{340jiang2020data} \\
Understanding & familiarity, story context & + & qualitative & \checkmark &  & medium & \cite{155bach2016telling} \\
Understanding & Visual expressiveness, annotations & + & qualitative & \checkmark &  & medium & \cite{155bach2016telling} \\
Understanding    & Data comic & +  & mixed-method  &     &   \checkmark   &  medium--large    &\cite{43wang2019comparing} \\
Usability & Interactive visualization  &+  & quantitative & \checkmark &  &medium  &\cite{70lunterova2019explorative} \\
Usability & Interface  & +  & qualitative & \checkmark &  & medium  &\cite{317tang2020design} \\
Usage (interface)  & Video and annotated visualization  & +  & mixed-method  & \checkmark  &  & small     &\cite{82zhi2019gameviews} \\
Usage & News visualizations & + & mixed-method  & \checkmark  &  & large &\cite{185de2018does} \\
Value  & News visualizations & + & mixed-method  & \checkmark  &  & large &\cite{185de2018does} \\

\bottomrule

\end{longtable}
\end{landscape}
